# Supplementary material for: Scalable Simulation of Realistic Volume Fraction Red Blood Cell Flows through Vascular Networks
Source: arXiv:1909.11085 source file (2019-09-23)
Supplement: Supplementary file 1 [file appendix.tex]

\appendix
\section{Appendix A\label{sec:app-a}}
